# Supplementary material for: Holoported Characters: Real-time Free-viewpoint Rendering of Humans from Sparse RGB Cameras
Source: arXiv:2312.07423 source file (2024-07-25)
Supplement: Supplementary file 1 [file additional_comparison.tex]

\begin{figure}
\centering
    \includegraphics[width=1.\linewidth]{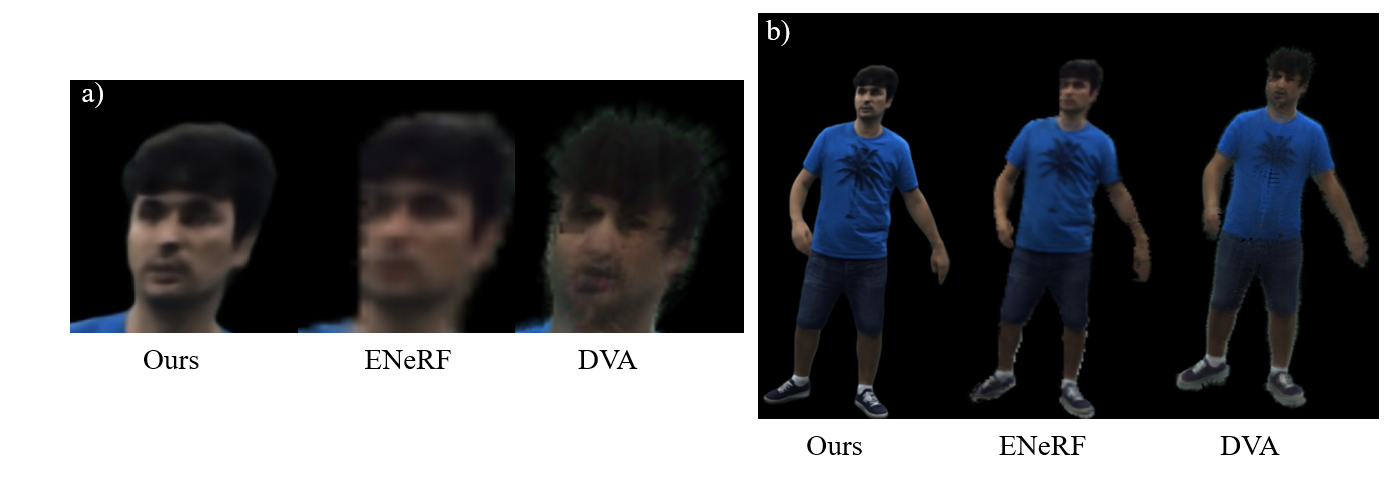}
    \vspace{-24pt}
    \caption{
    \textbf{Additional Comparison with Other Subjects}
  .
    }
    \label{fig:additonal_comp}
\end{figure}
